# Supplementary material for: Isotropic SGD: a Practical Approach to Bayesian Posterior Sampling
Source: arXiv:2006.05087 source file (2020-06-09)
Supplement: Supplementary file 1 [file appendix.tex]

\documentclass{article}

\usepackage[]{neurips_2020}

\usepackage{algorithm}
\usepackage[noend]{algpseudocode}

\usepackage[utf8]{inputenc} % allow utf-8 input
\usepackage[T1]{fontenc}    % use 8-bit T1 fonts
\usepackage{url}            % simple URL typesetting
\usepackage{amsfonts}       % blackboard math symbols
\usepackage{nicefrac}       % compact symbols for 1/2, etc.

\usepackage{microtype}
\usepackage[pdftex]{graphicx}
\usepackage{booktabs}
\usepackage{amsmath}

\usepackage{pgfplots}
\pgfplotsset{width=8cm,height=5cm,compat=1.9}
\newlength\figureheight
\newlength\figurewidth

\usepackage{subfig}
\usepackage{amsmath}

\usepackage{amssymb}
\usepackage{amsfonts}
\usepackage{amstext}
\usepackage{xcolor}
\usepackage{xspace}
\usepackage{appendix}
\usepackage[bottom]{footmisc}
\usepackage[breaklinks]{hyperref}
\usepackage{cleveref}

\makeatletter

\newcommand*{\addFileDependency}[1]{% argument=file name and extension
  \typeout{(#1)}
  \@addtofilelist{#1}
  \IfFileExists{#1}{}{\typeout{No file #1.}}
}

\makeatother

\newcommand*{\myexternaldocument}[1]{%
\externaldocument{#1}%
\addFileDependency{#1.tex}%
\addFileDependency{#1.aux}%
}

\usepackage{xr}
\myexternaldocument{main}

\crefname{appsec}{Appendix}{Appendices}
\crefname{appsubsec}{Appendix}{Appendices}
\crefalias{section}{appsec}
\crefalias{subsection}{appsubsec}

% \renewcommand*{\thesubsubsection}{\roman{subsubsection}}

% \icmltitlerunning{Appendix}
\input{notation.tex}

% \title{Isotropic SGD: a Practical Approach to Bayesian Posterior Sampling}
\title{Isotropic SGD: Practical Bayesian Posterior Sampling\\ Supplementary Material}

\author{Anonymous}

\begin{document}
\maketitle
\crefalias{section}{appsec}
\crefalias{subsection}{appsubsec}

\section{\mcmc Through the Lenses of Langevin Dynamics}
\label{appa}
\input{theoreticalres.tex}

\section{\isgd method proofs and details}
\label{appb}
\input{isgdmethod.tex}

%\section{Alpha Stable parameter estimation}
%\label{appc}
%\input{alphaestim.tex}

\section{Toy Model}
\label{appd}
\input{apptoymodel.tex}

\section{Experimental Methodology}
\label{appc}
\input{metodology.tex}

\bibliographystyle{abbrv}
\bibliography{biblio_appendix}

\newpage
\clearpage
\newpage

\nocite*{}
\clearpage
\end{document}
